# Supplementary material for: Self-supervised Visual Attribute Learning for Fashion Compatibility
Source: arXiv:2008.00348 source file (2021-08-12)
Supplement: Supplementary file 2 [file fig_supp_tsne_RGB.tex]

\begin{figure*}[h]
	\centering
% 	\begin{subfigure}[t]{1.0\textwidth}
    % \hspace{-1.0in}
    \includegraphics[width=\linewidth]{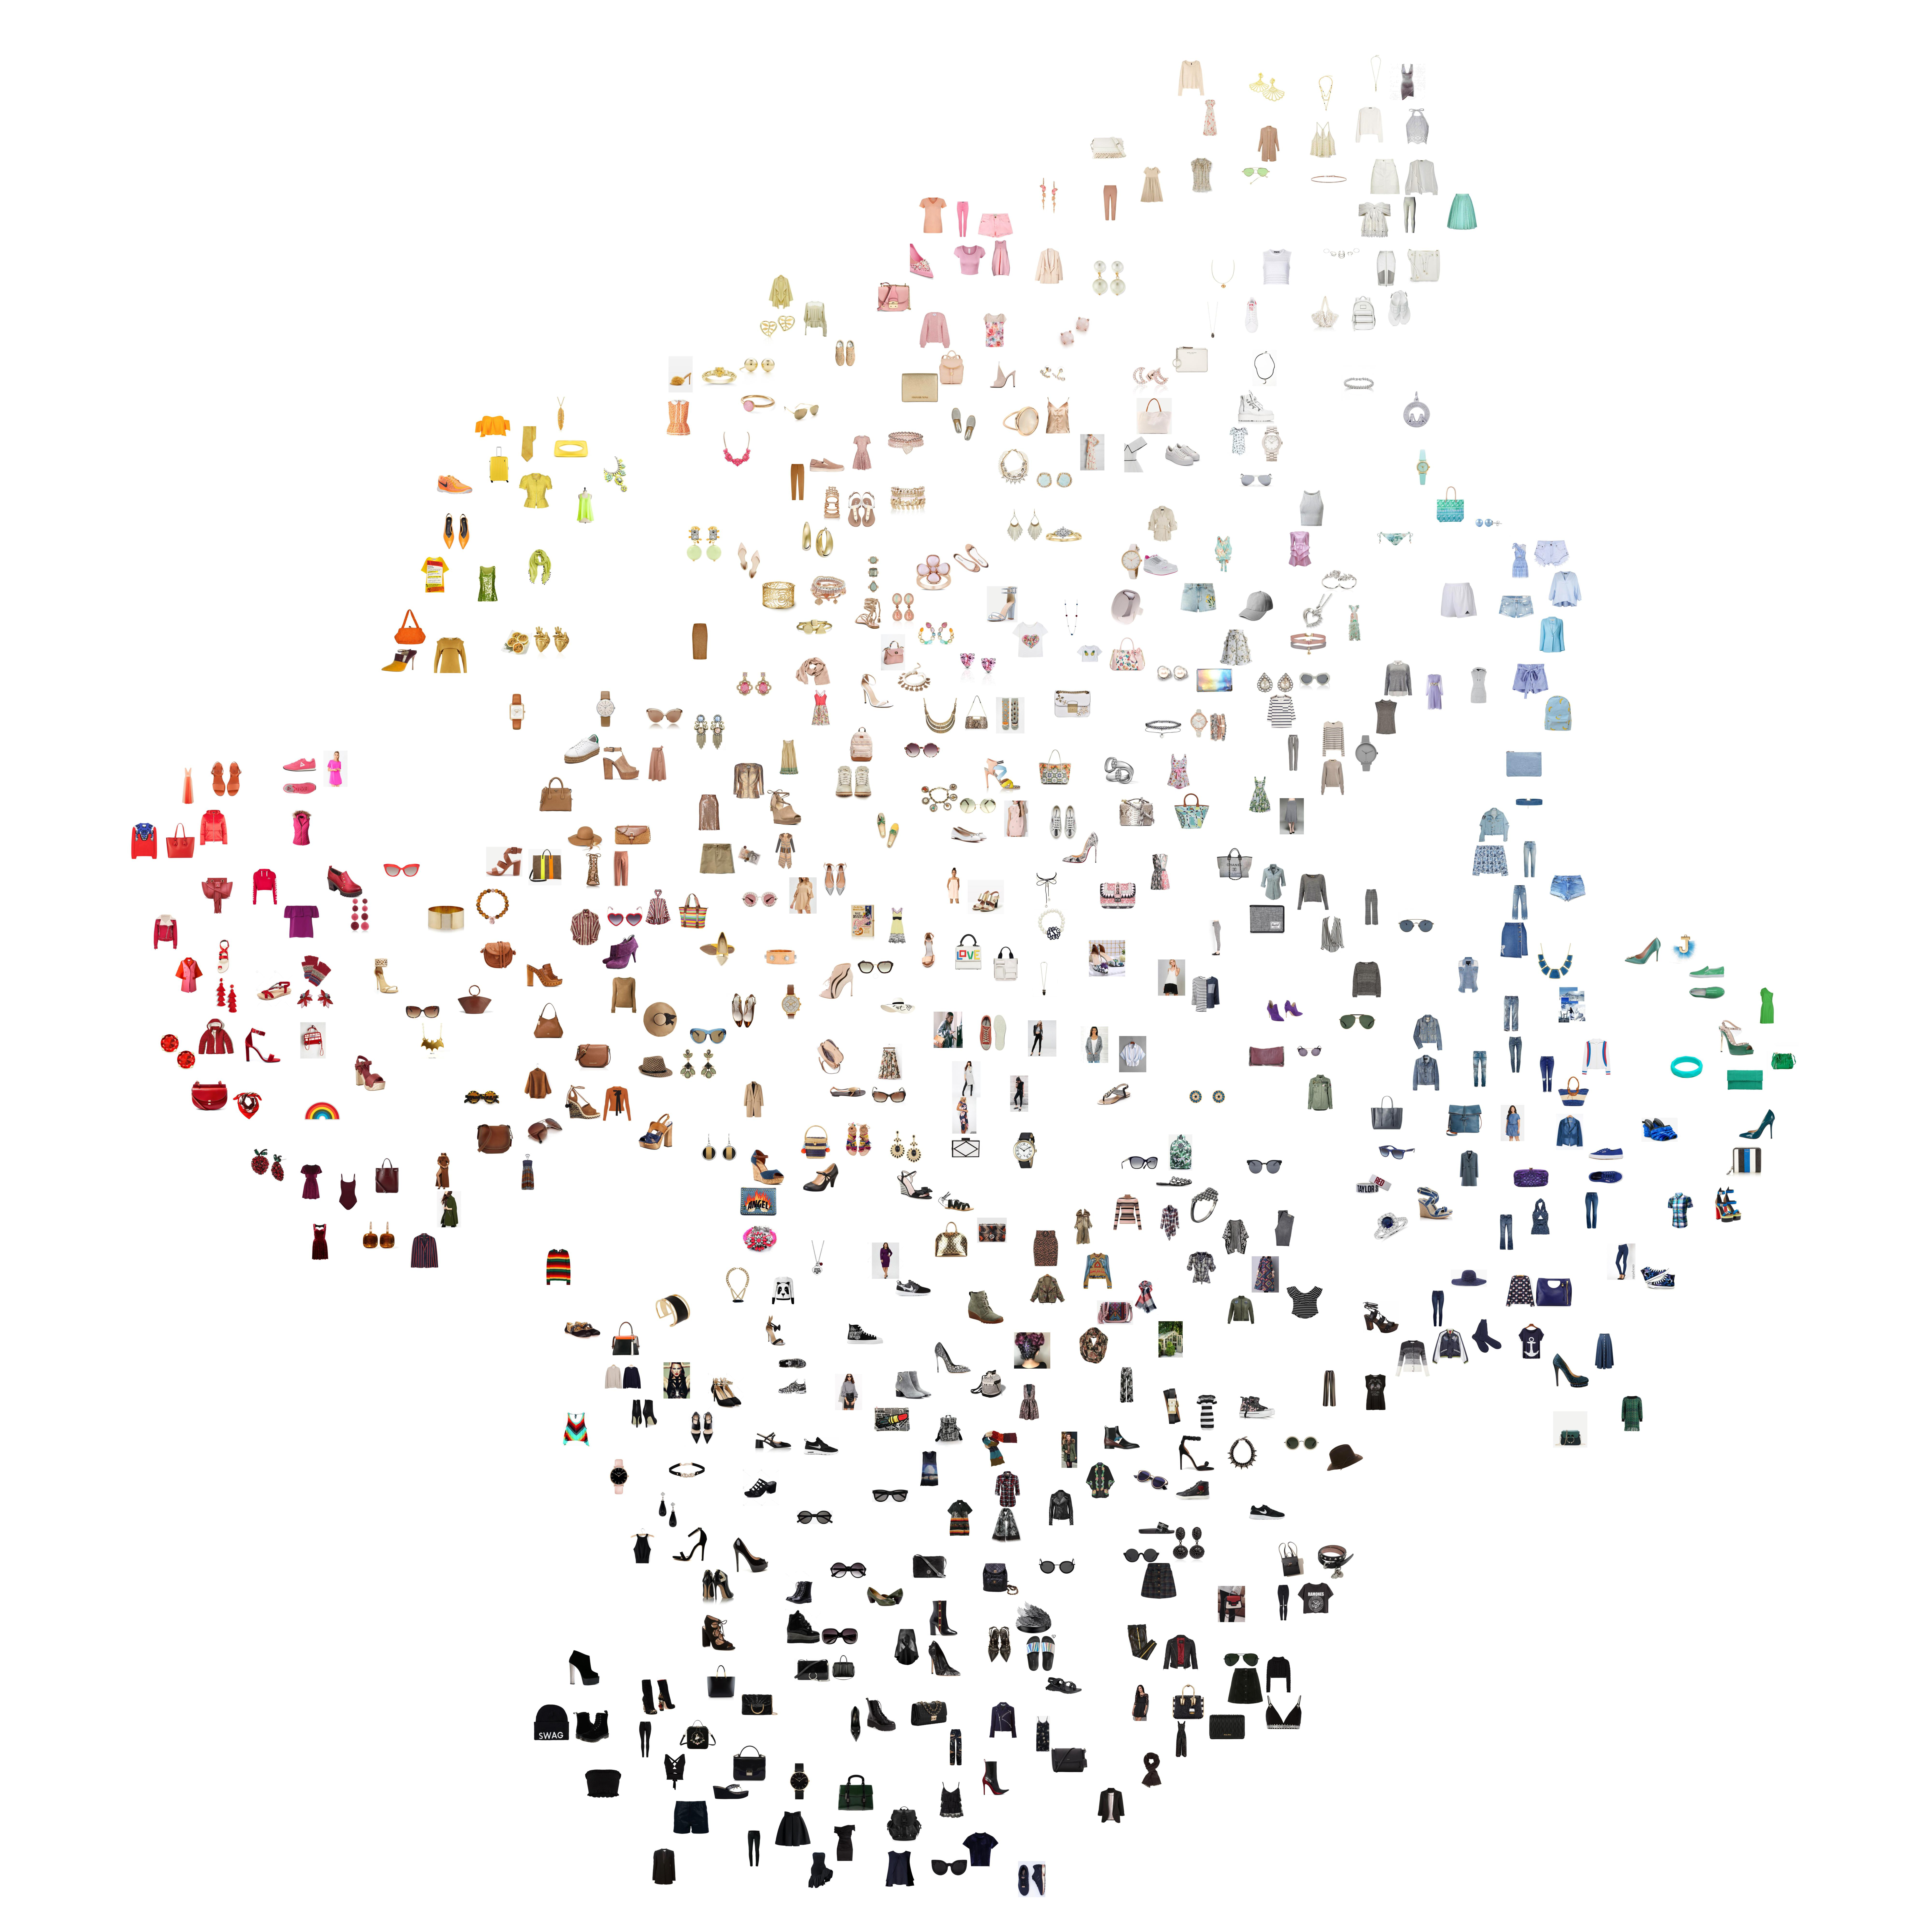}
    \caption{t-SNE visualization of features from predicting RGB histrograms (ours).}
	\label{fig:supp_tsne_rgb}
	\vspace{-4mm}
\end{figure*}
