# Supplementary material for: Self-supervised Visual Attribute Learning for Fashion Compatibility
Source: arXiv:2008.00348 source file (2021-08-12)
Supplement: Supplementary file 8 [file supp_table_others.tex]

% \begin{SCtable}
% % \centering
% \caption{Cross dataset experiments. We train a model on the Fashion-Gen dataset and test it on the Polyvore dataset. We report the performances of (a)  self-supervised learning baselines and (b) ours. Our method is able to generalize across different datasets.}

% % \begin{subtable}[t]{0.5\textwidth}
% % \caption{Cross Dataset Evaluation}
% \begin{tabular}{|ll|c|c|}
% \hline
%  & & \multicolumn{2}{c|}{Fashion-Gen $\rightarrow$ Polyvore} \\
%  \hline
%     &Method & Comp. AUC & FITB acc.   \\
% \hline
% \hline
% (a)   & ID~\cite{wu2018unsupervised} & 0.71 & 45.5 \\
%   &    Local Agg.~\cite{zhuang2019local} & 0.73 & 46.5\\
%     \hline
% (b)&    RGB & 0.76 & 48.1  \\ 
%     % SLPD & 0.80 & 52.6 \\
%     % TD & 0.76 & 49.9 \\
%  &   RGB+SLPD & 0.81 & 54.0 \\
%   &  RGB+SLPD+TD & \textbf{0.82} & \textbf{54.2} \\
% % \hline
% \hline
% \end{tabular}
% % \end{subtable}

% \label{exp:tab_1}
% \end{SCtable}

\begin{table}[h]
\centering

\resizebox{0.49\textwidth}{!}{\begin{tabular}{|l|c|c|c|}
\hline
 & \multicolumn{2}{c|}{Polyvore Outfits} & Capsule \\
\hline
    Method & Comp. AUC & FITB acc. & Comp. AUC  \\
\hline
% \hline
    RGB & 0.77 $\pm$ 0 & 47.2 $\pm$ 0.23 & 23.3 $\pm$ 0.1\\ 
    SLPD & 0.83 $\pm$ 0 & 54.6 $\pm$ 0.52 & 27.7 $\pm$ 0.25\\
    TD & 0.77 $\pm$ 0  & 50.3 $\pm$ 0.36 & 25.2 $\pm$ 0.37 \\
    RGB+SLPD & 0.83  $\pm$ 0 & 55.4 $\pm$ 0.35 & 27.7 $\pm$0.15 \\
    RGB+SLPD+TD & 0.84 $\pm$ 0 & 55.8 $\pm$ 0.15 & 27.9 $\pm$ 0.15 \\
% \hline
\hline
\end{tabular}}
\caption{Standard deviation over three runs on Polyvore Outfits~\cite{vasileva2018learning} for the fashion compatibility task.}
\label{exp:supp_std}
\vspace{-4mm}
\end{table}
